# Supplementary material for: Effective Attention Sheds Light On Interpretability
Source: arXiv:2105.08855 source file (2021-05-18)
Supplement: Supplementary file 1 [file tags_appendix.tex]

\begin{figure*}[t]
    \centering
    \subfloat[Standard attention.]{\includegraphics[width=\the\textwidth]{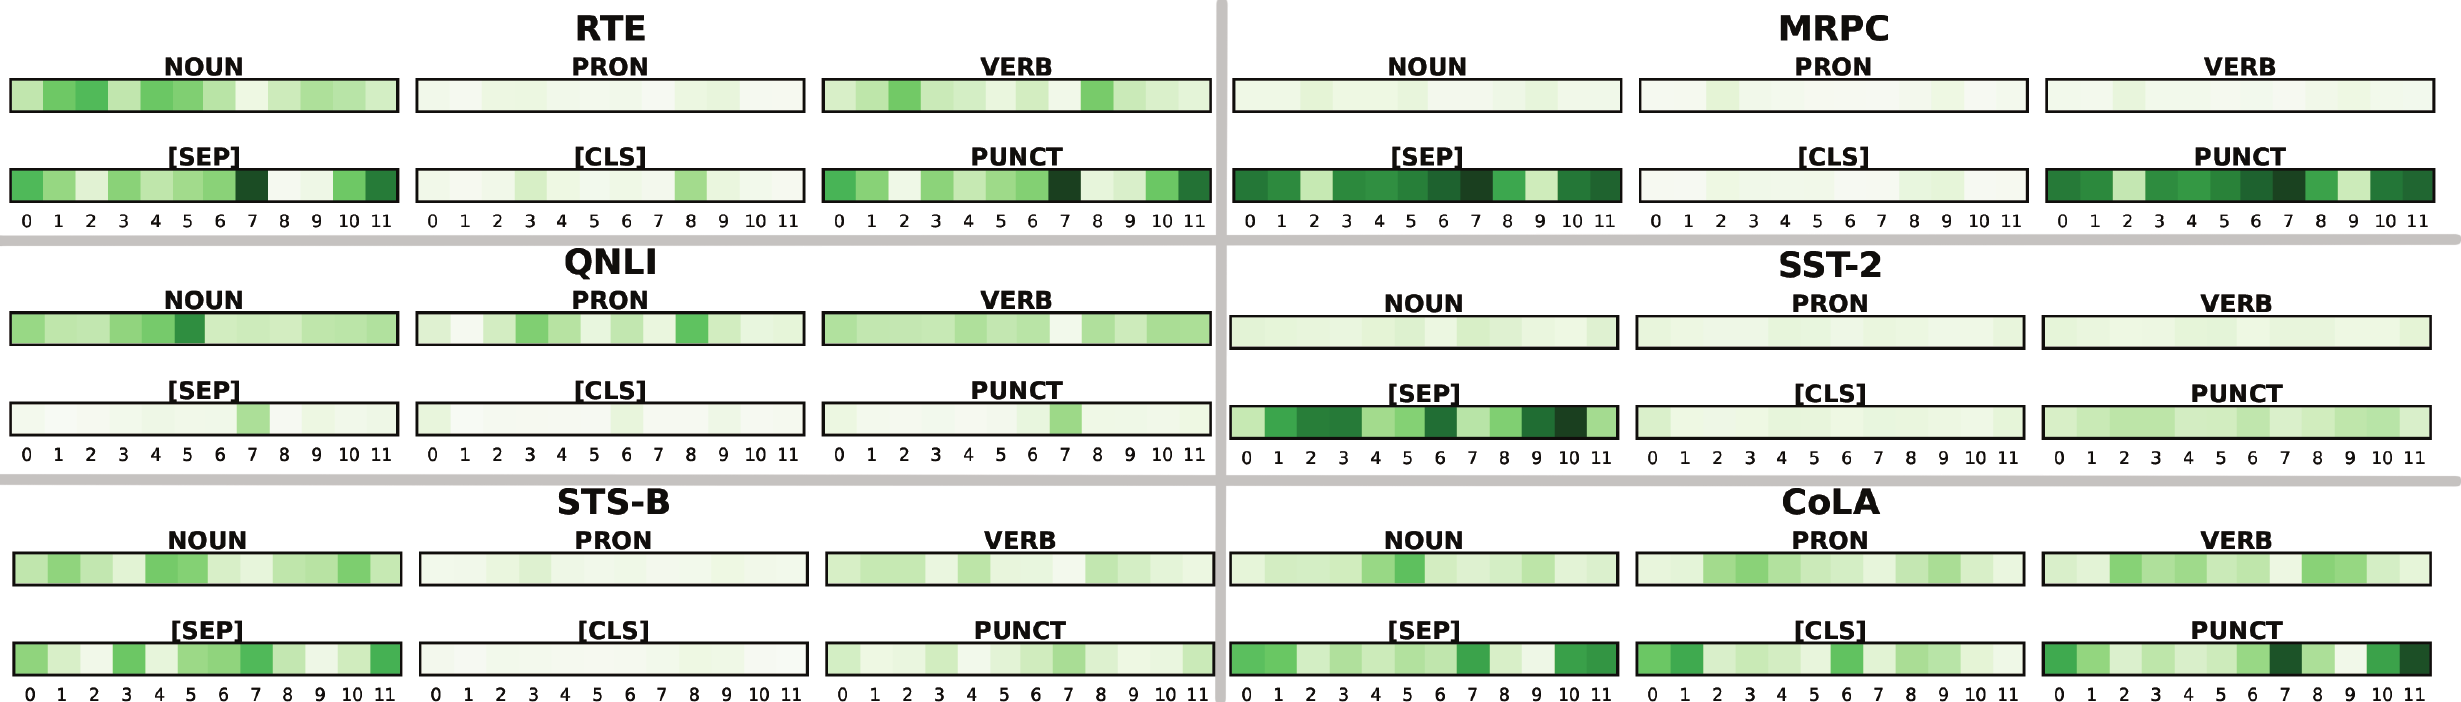} }
    \qquad
    \subfloat[Effective Attention]{\includegraphics[width=\the\textwidth]{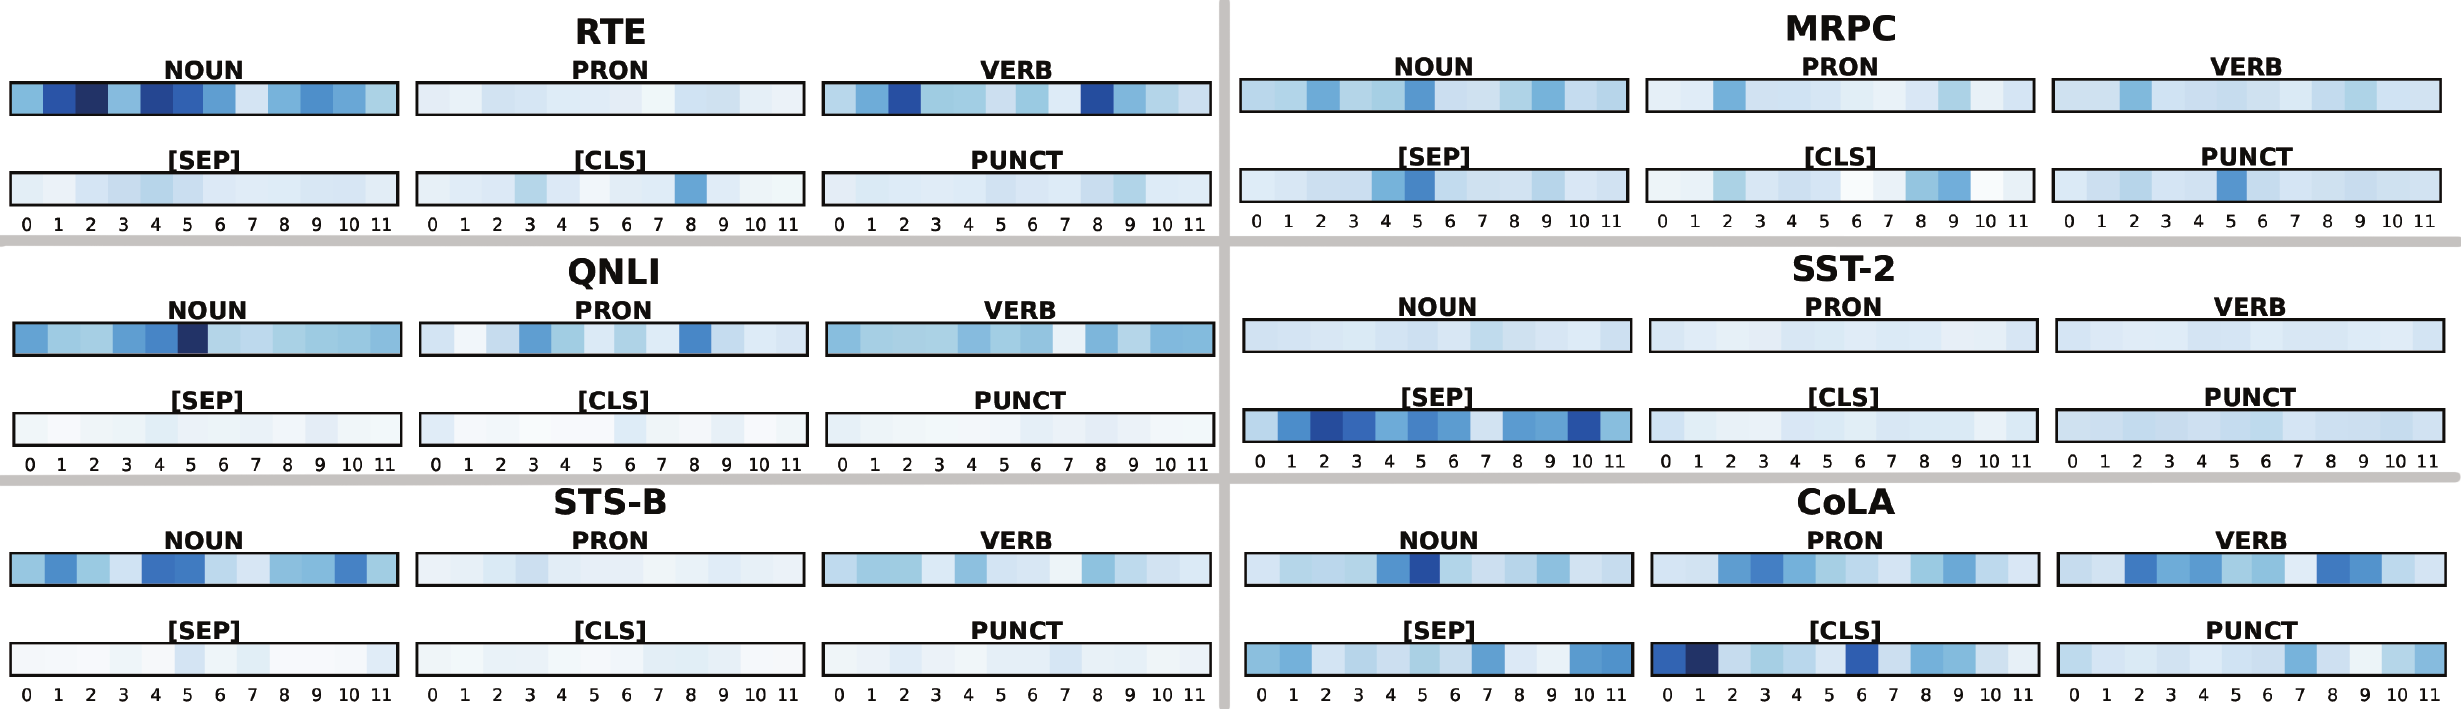} }
    \caption{Per-task attention weights corresponding to the \clstoken token averaged over dataset examples from the final layer.}
    \label{fig:tags}
\end{figure*}
